# Supplementary material for: Projective Preferential Bayesian Optimization
Source: arXiv:2002.03113 ancillary file (2020-08-14)
Supplement: Supplementary file 1 [file Supplement.pdf]

# Supplementary Material
## *Projective Preferential Bayesian Optimization*

**Petrus Mikkola** [1] **Milica Todorović** [2] **Jari Järvi** [2] **Patrick Rinke** [2] **Samuel Kaski** [1 3]

— *The source code written in Python is available at* https://github.com/AaltoPML/PPBO —

This supplementary material provides more details about the technicalities and implementation of the Projective Preferential Bayesian Optimization framework [1]. The document is divided into eight subsections that discuss the projective preferential feedback, the derivation of the likelihood, the choice of Monte-Carlo sampling distribution in the likelihood, the model selection, the Gaussian process covariance matrix, the optimization of acquisition functions, the derivatives of the log-scaled posterior $T$, and the numerical experiments, respectively.

### Projective preferential feedback

Given a projective preferential query, $(\boldsymbol{\xi}, \mathbf{x}) \in \Xi \times \mathcal{X} \subset \mathbb{R}^D \times \mathbb{R}^D$, the projective preferential feedback is obtained as *a minimizer over the possible scalar projections*,

$$\alpha^* = \operatorname*{argmin}_{\alpha \in \mathcal{I}_{\boldsymbol{\xi}}} f(\alpha\boldsymbol{\xi} + \mathbf{x}),$$

where $\mathcal{I}_{\boldsymbol{\xi}} \equiv \{\alpha \in \mathbb{R} | \alpha\boldsymbol{\xi} + \mathbf{x} \in \mathcal{X}\}$. The set $\mathcal{I}_{\boldsymbol{\xi}}$ is independent of the reference vector $\mathbf{x}$, since $\mathbf{x}$ has the property that $x_d = 0$ for all $d \in \{1, ..., D\}$ such that $\xi_d \neq 0$. In fact, it holds that $\mathcal{I}_{\boldsymbol{\xi}} = [\max_{\xi_d \neq 0}\{\frac{a_d}{\xi_d}\}, \min_{\xi_d \neq 0}\{\frac{b_d}{\xi_d}\}]$.

In principle, the minimizer $\alpha^*$ is not necessarily unique. For instance, $\alpha^* = \{-2, 2\}$ when $\mathcal{X} = [-2, 2]$, $f(\mathbf{x}) = -x_1^2 - x_2^2$, $\boldsymbol{\xi} = (1, 1)$ and $\mathbf{x} = (0, 0)$. However, in practice, the minimizer $\alpha^*$ is always unique. For instance, when $f$ is a numerical test function, then $\alpha^*$ is obtained by using a numerical optimization algorithm that outputs a unique value $\alpha^*$. In theory, the non-uniqueness issue can be also fixed by assuming that *ties are broken non-arbitrarily*, that is, $(\boldsymbol{\xi}, \mathbf{x}) \mapsto \operatorname{argmin}_{\alpha \in \mathcal{I}_{\boldsymbol{\xi}}} f(\alpha\boldsymbol{\xi} + \mathbf{x})$ is forced to be a single-valued function through a non-stochastic *tiebreaker-policy*. For example, we may follow the tiebreaker-policy that picks the smallest element from the set of minimizers.

### Likelihood

Given two alternatives $(\alpha\boldsymbol{\xi} + \mathbf{x}), (\beta\boldsymbol{\xi} + \mathbf{x}) \in \mathcal{X}$, we assume that $\alpha\boldsymbol{\xi} + \mathbf{x} \succ \beta\boldsymbol{\xi} + \mathbf{x}$, if and only if $f(\alpha\boldsymbol{\xi} + \mathbf{x}) + W(\alpha) > f(\beta\boldsymbol{\xi} + \mathbf{x}) + W(\beta)$, where $W$ is a *Gaussian white noise process* with zero-mean and autocorrelation $\mathbb{E}(W(t)W(t+\tau)) = \sigma^2$ if $\tau = 0$, and zero otherwise. We would like to find the likelihood for an observation $(\alpha, (\boldsymbol{\xi}, \mathbf{x}))$ that corresponds to uncountably infinite pairwise comparisons, $\alpha\boldsymbol{\xi} + \mathbf{x} \succ \beta\boldsymbol{\xi} + \mathbf{x}$ for $\beta \neq \alpha$. For each comparison we condition on $W(\alpha)$, so the following probability measure (for fixed $w \in \mathbb{R}$) should be interpreted as a *regular conditional probability*,

$$\begin{aligned} &\mathrm{P}\left(\alpha\boldsymbol{\xi} + \mathbf{x} \succ \beta\boldsymbol{\xi} + \mathbf{x} \mid W(\alpha) = w\right) = \mathrm{P}\left(W(\beta) > f(\beta\boldsymbol{\xi} + \mathbf{x}) - f(\alpha\boldsymbol{\xi} + \mathbf{x}) - w \mid W(\alpha) = w\right) \\ &= \mathrm{P}\left(\frac{W(\beta)}{\sigma} > \frac{f(\beta\boldsymbol{\xi} + \mathbf{x}) - f(\alpha\boldsymbol{\xi} + \mathbf{x}) - w}{\sigma} \Big| W(\alpha) = w\right) = 1 - \Phi\left(\frac{f(\beta\boldsymbol{\xi} + \mathbf{x}) - f(\alpha\boldsymbol{\xi} + \mathbf{x}) - w}{\sigma}\right), \end{aligned}$$

where $\Phi$ is the cumulative distribution function of the standard normal distribution. Hence, for a comparison we have

$$\mathrm{P}\left(\alpha\boldsymbol{\xi} + \mathbf{x} \succ \beta\boldsymbol{\xi} + \mathbf{x}\right) = \int_{-\infty}^{\infty} \mathrm{P}\left(\alpha\boldsymbol{\xi} + \mathbf{x} \succ \beta\boldsymbol{\xi} + \mathbf{x} \mid W(\alpha) = w\right) \mathcal{N}(w|0, \sigma^2) dw = 1 - [\Phi * \phi]\left(\frac{f(\beta\boldsymbol{\xi} + \mathbf{x}) - f(\alpha\boldsymbol{\xi} + \mathbf{x})}{\sigma}\right),$$

[1]Helsinki Institute for Information Technology HIIT, Department of Computer Science, Aalto University, Espoo, Finland [2]Department of Applied Physics, Aalto University, Espoo, Finland [3]The University of Manchester, UK. Correspondence to: Petrus Mikkola <petrus.mikkola@aalto.fi>, Samuel Kaski <samuel.kaski@aalto.fi>.

*Proceedings of the $37^{th}$ International Conference on Machine Learning*, Online, PMLR 119, 2020. Copyright 2020 by the author(s).

where $\phi$ is the probability density of the standard normal distribution and $*$ is the convolution operator. In the last equation, the change of variables $v = \sigma w$ is used in the integration. For infinite comparisons, we first consider a finite number of comparisons $m$. By the independence of $W(\beta)$ (uncorrelated jointly Gaussian, thus the independence follows), we have

$$\mathrm{P}\left(\alpha\boldsymbol{\xi} + \mathbf{x} \succ \beta_1\boldsymbol{\xi} + \mathbf{x}, ..., \alpha\boldsymbol{\xi} + \mathbf{x} \succ \beta_m\boldsymbol{\xi} + \mathbf{x}\right) = \prod_{j=1}^{m} \left(1 - [\Phi * \phi]\left(\frac{f(\beta_j\boldsymbol{\xi} + \mathbf{x}) - f(\alpha\boldsymbol{\xi} + \mathbf{x})}{\sigma}\right)\right).$$

By letting the number of points $m$ in an increasing sequence $\beta_1, ..., \beta_m$ of the partition of the interval $\mathcal{I}_{\boldsymbol{\xi}} \backslash \{\alpha\}$ to approach infinity, we can interpret this as a Volterra (product) integral

$$\prod_{\beta \in \mathcal{I}_{\boldsymbol{\xi}} \backslash \{\alpha\}} \left(1 - [\Phi * \phi]\Big(\frac{f(\beta\boldsymbol{\xi} + \mathbf{x}) - f(\alpha\boldsymbol{\xi} + \mathbf{x})}{\sigma}\Big) d\beta\right) = \exp\left(-\int_{\mathcal{I}_{\boldsymbol{\xi}} \backslash \{\alpha\}} [\Phi * \phi]\Big(\frac{f(\beta\boldsymbol{\xi} + \mathbf{x}) - f(\alpha\boldsymbol{\xi} + \mathbf{x})}{\sigma}\Big) d\beta\right)$$
$$= \exp\left(-\int_{\mathcal{I}_{\boldsymbol{\xi}}} [\Phi * \phi]\Big(\frac{f(\beta\boldsymbol{\xi} + \mathbf{x}) - f(\alpha\boldsymbol{\xi} + \mathbf{x})}{\sigma}\Big) d\beta\right).$$

This corresponds to the likelihood of an observation $(\alpha, (\boldsymbol{\xi}, \mathbf{x}))$.

### Monte-Carlo sampling distribution

Here, we give more details about the form of sampling distribution used in a Monte-Carlo integral that approximates the likelihood.

The pseudo-observations $(\beta_j\boldsymbol{\xi})_j^m$ for $j = 1, ..., m$ are sampled from the family of truncated generalized normal (TGN) distributions (see e.g. [3]), since it provides a continuous transformation from the uniform distribution to the truncated normal distribution such that the locations of distributions can be specified. The principal idea is to concentrate the pseudo-observations more densely around the optimal value $\alpha\boldsymbol{\xi}$ as time proceeds (measured as a number of passed queries).

More precisely, a sequence $(\beta_j)_{j=1}^m$ is sampled independently and identically from the probability density function,

$$p_\beta(x) = \frac{\phi(\frac{x-\alpha}{\tilde{\sigma}(\gamma)})\mathbb{I}_{\{x \in [\min \mathcal{I}_{\boldsymbol{\xi}}, \max \mathcal{I}_{\boldsymbol{\xi}}]\}}}{\tilde{\sigma}(\gamma)\big(\Phi(\frac{\max \mathcal{I}_{\boldsymbol{\xi}} - \alpha}{\tilde{\sigma}(\gamma)}) - \Phi(\frac{\min \mathcal{I}_{\boldsymbol{\xi}} - \alpha}{\tilde{\sigma}(\gamma)})\big)}, \tag{1}$$

where $\phi(x) \equiv \frac{\gamma}{2\Gamma(1/\gamma)} \exp(-|x|^\gamma)$ is the density of the centralized reduced generalized normal distribution (with the form parameter $\gamma$), $\Phi$ its the cumulative distribution function of the standard normal distribution, and $\tilde{\sigma}(\cdot)$ is a positive function of the parameter $\gamma$. The latter function describes the shape of the distribution, and we assume that it takes the following form: $\tilde{\sigma}(\gamma) = \Gamma(\gamma)\frac{|\max \mathcal{I}_{\boldsymbol{\xi}} - \min \mathcal{I}_{\boldsymbol{\xi}}|}{10}$. Note that the location parameter is set to the optimal value $\alpha$, so that the pseudo-observations are concentrated around that. The form parameter $\gamma$ is tied to the current iteration ($n$) of the Bayesian optimization loop. At the beginning ($n = 1$) we set $\gamma$ to some relatively high value, say $\gamma_1 = 5$. As $n \to \infty$, the density (1) approaches the truncated normal distribution, since we force $\gamma_n \to 2$. For instance, this can be achieved by setting $\gamma_n \equiv 3/(\max\{n + 1 - D, 1\})^s + 2$, where the parameter $s \in (0, 1]$ controls the speed of the transformation. In the numerical experiments, we used $s = 0.4$. Given $(\beta_j)_{j=1}^m$, the pseudo-observations can be obtained by scaling, $(\beta_j\boldsymbol{\xi})_{j=1}^m$.

### Hyperparameter optimization

We adapt the *type II maximum likelihood scheme*. The hyperparameters, $\boldsymbol{\theta} = (\sigma, \sigma_f, l)$ , are optimized by maximizing the marginal likelihood $\mathrm{P}(\mathcal{D}) = \mathrm{P}(\mathcal{D}|\boldsymbol{\theta})$, which can be expressed as

$$\mathrm{P}(\mathcal{D}|\boldsymbol{\theta}) = \exp(T(\mathbf{f}_{\mathrm{MAP}}))\Big(\sqrt{(2\pi)^D|\Sigma|}\mathrm{P}(\mathbf{f}_{\mathrm{MAP}}|\mathcal{D})\Big)^{-1},$$

since the functional $T$ can be written as,

$$T(\mathbf{f}) = \log\Big(\sqrt{(2\pi)^D|\Sigma|}\mathrm{P}(\mathbf{f}|\mathcal{D})\mathrm{P}(\mathcal{D})\Big).$$

From the Laplace approximation we have that $\mathbf{f}|\mathcal{D}$ is distributed as $\mathcal{N}\big(\mathbf{f}_{\mathrm{MAP}}, (\Sigma^{-1} + \Lambda)^{-1}\big)$. Thus, the marginal likelihood simplifies to the expression,

$$\mathrm{P}(\mathcal{D}|\boldsymbol{\theta}) = \exp(T(\mathbf{f}_{\mathrm{MAP}}))|I + \Sigma\Lambda|^{-\frac{1}{2}}.$$

After the kernel $k$ has been fixed, the gradient of the marginal likelihood can be derived analytically. Gradient-based methods can be used in the optimization of the marginal likelihood. Due to numerical instabilities, the logarithm of the marginal likelihood may be preferred,

$$\log \mathrm{P}(\mathcal{D}|\boldsymbol{\theta}) = T(\mathbf{f}_{\text{MAP}}) - \frac{1}{2}\log|I + \Sigma\Lambda|.$$

### Covariance matrix

The covariance matrix $\Sigma$ has a high condition number. We used a *shrinkage method* as described in [2] to reduce the condition number of $\Sigma$. There is available an implementation of this method in the Python's *scikit-learn* -package: https://scikit-learn.org/stable/modules/covariance.html#shrunk-covariance.

### Optimization of acquisition functions

Since the reference vector $\mathbf{x}$ has the property that $x_d = 0$ for all $d \in \{1, ..., D\}$ such that $\xi_d \neq 0$, we have to take that into account in the optimization of acquisition functions (this applies to PPBO-EI, PPBO-EXR, and PPBO-EXT). Along the same line as the preferential coordinate descent (PPBO-PCD), we rotate the non-zero coordinates of $\boldsymbol{\xi}$ in a cyclical order for each query. In particular, we set $\boldsymbol{\xi} = (\xi_1, ..., \xi_{d-1}, 0, \xi_{d+1}, ..., \xi_D)$, and rotate $d$ in a cyclical order for each query. This means that the reference vector is $\mathbf{x} = (0, ..., 0, x_d, 0, ..., 0)$. Then, the pair of vectors $(\boldsymbol{\xi}, \mathbf{x})$ (that is the values $\xi_1, ..., \xi_{d-1}, \xi_{d+1}, ..., \xi_D$ and $x_d$) are optimized by maximizing the chosen acquisition function as described in the paper.

This optimization, in principle, can be carried out by using any numerical global optimization algorithm. We found that Bayesian optimization[1] is a good option for that, since it is prudent in the number of acquisition function evaluations. Thus, it speeds up the optimization at the cost of finding only approximately optimal global maximum. In the numerical experiments, we limit the number of Bayesian optimization iterations to 30.

In the random acquisition (PPBO-RAND) everything is random: the number of non-zero coordinates ($N \sim$ Unif$(\{1, .., D\})$), what are the non-zero coordinates (uniformly random combination $\binom{D}{N}$), and the values of the non-zero coordinates (each coordinate sampled from Unif$(0, 1)$).

### Gradient and Hessian of the functional T

For notational convenience, define

$$\Delta_{i,j}(\mathbf{f}) \equiv \frac{f(\beta_j^i \boldsymbol{\xi}^i + \mathbf{x}^i) - f(\alpha^i \boldsymbol{\xi}^i + \mathbf{x}^i)}{\sigma}.$$

So, that means,

$$\frac{\partial}{\partial f(\alpha^i \boldsymbol{\xi}^i + \mathbf{x}^i)} \Delta_{i,j}(\mathbf{f}) = -\frac{1}{\sigma}$$
$$\frac{\partial}{\partial f(\beta_j^i \boldsymbol{\xi}^i + \mathbf{x}^i)} \Delta_{i,j}(\mathbf{f}) = \frac{1}{\sigma}.$$

Recall the form of the functional $T$,

$$T(\mathbf{f}) \approx -\frac{1}{2}\mathbf{f}^\top \Sigma^{-1}\mathbf{f} - \frac{1}{m}\sum_{i=1}^{N}\sum_{j=1}^{m}[\Phi * \phi]\big(\Delta_{i,j}(\mathbf{f})\big).$$

We need the two first derivatives of the convolution $[\Phi * \phi]$. These are $[\Phi * \phi]'(x) = \phi_2(x)$ and $[\Phi * \phi]''(x) = -\frac{x}{2}\phi_2(x)$, where $\phi_2$ is the density function of $N(0, \sqrt{2}^2)$.

<u>The gradient of $T$:</u>

[1] We used a Python open-source library, *GPyOpt*, for Bayesian Optimization [4]. The library is developed by the Machine Learning group of the University of Sheffield.

$\nabla T = -\Sigma^{-1}\mathbf{f} + \boldsymbol{\beta}$, and the vector $\boldsymbol{\beta}$ is given by the following partial derivatives:

$$\frac{\partial}{\partial f(\alpha^i \boldsymbol{\xi}^i + \mathbf{x}^i)} - \frac{1}{m}\sum_{i=1}^{N}\sum_{j=1}^{m}[\Phi * \phi]\big(\Delta_{i,j}(\mathbf{f})\big) = \frac{1}{\sigma m}\sum_{j=1}^{m}[\Phi * \phi]'\big(\Delta_{i,j}(\mathbf{f})\big) = \frac{1}{\sigma m}\sum_{j=1}^{m}\phi_2\big(\Delta_{i,j}(\mathbf{f})\big)$$

$$\frac{\partial}{f(\beta_j^i \boldsymbol{\xi}^i + \mathbf{x}^i)} - \frac{1}{m}\sum_{i=1}^{N}\sum_{j=1}^{m}[\Phi * \phi]\big(\Delta_{i,j}(\mathbf{f})\big) = -\frac{1}{\sigma m}[\Phi * \phi]'\big(\Delta_{i,j}(\mathbf{f})\big) = -\frac{1}{\sigma m}\phi_2\big(\Delta_{i,j}(\mathbf{f})\big).$$

<u>The Hessian of $T$:</u>

$\nabla\nabla T = -\Sigma^{-1} + \Lambda$, and a symmetric matrix $\Lambda$ is given by the following partial derivatives:

$$\frac{\partial^2}{\partial f(\alpha^i \boldsymbol{\xi}^i + \mathbf{x}^i) f(\alpha^i \boldsymbol{\xi}^i + \mathbf{x}^i)} = \frac{\partial}{\partial f(\alpha^i \boldsymbol{\xi}^i + \mathbf{x}^i)}\frac{1}{\sigma m}\sum_{j=1}^{m}[\Phi * \phi]'\big(\Delta_{i,j}(\mathbf{f})\big)$$
$$= -\frac{1}{\sigma^2 m}\sum_{j=1}^{m}[\Phi * \phi]''\big(\Delta_{i,j}(\mathbf{f})\big) = \frac{1}{2\sigma^2 m}\sum_{j=1}^{m}\Delta_{i,j}(\mathbf{f})\phi_2\big(\Delta_{i,j}(\mathbf{f})\big)$$

$$\frac{\partial^2}{\partial f(\alpha^i \boldsymbol{\xi}^i + \mathbf{x}^i) f(\beta_j^i \boldsymbol{\xi}^i + \mathbf{x}^i)} = \frac{\partial}{\partial f(\beta_j^i \boldsymbol{\xi}^i + \mathbf{x}^i)}\frac{1}{\sigma m}\sum_{j=1}^{m}[\Phi * \phi]'\big(\Delta_{i,j}(\mathbf{f})\big)$$
$$= \frac{1}{\sigma^2 m}[\Phi * \phi]''\big(\Delta_{i,j}(\mathbf{f})\big) = -\frac{1}{2\sigma^2 m}\Delta_{i,j}(\mathbf{f})\phi_2(\Delta_{i,j}(\mathbf{f}))$$

$$\frac{\partial^2}{\partial f(\beta_j^i \boldsymbol{\xi}^i + \mathbf{x}^i) f(\beta_j^i \boldsymbol{\xi}^i + \mathbf{x}^i)} = \frac{\partial}{\partial f(\beta_j^i \boldsymbol{\xi}^i + \mathbf{x}^i)} - \frac{1}{\sigma m}[\Phi * \phi]'\big(\Delta_{i,j}(\mathbf{f})\big)$$
$$= -\frac{1}{\sigma^2 m}[\Phi * \phi]''\big(\Delta_{i,j}(\mathbf{f})\big) = \frac{1}{2\sigma^2 m}\Delta_{i,j}(\mathbf{f})\phi_2\big(\Delta_{i,j}(\mathbf{f})\big).$$

## Numerical experiments

In the numerical experiments, we consider a following variant of a dueling-Thompson sampling acquisition strategy described in Subsection 3.3. of [5]. In PBO-DTS, we choose

$$\mathbf{x}_{next} = \operatorname*{argmax}_{\mathbf{x}\in\mathcal{X}} h_{\tilde{f}}(\mathbf{x}), \qquad where \quad h_{\tilde{f}}(\mathbf{x}) := \int_{\mathcal{X}} \pi_{\tilde{f}}([\mathbf{x}, \mathbf{x}']; \mathcal{D}_j) d\mathbf{x}'.$$

Given $(\tilde{f}, \mathbf{x})$, the integral $h_{\tilde{f}}(\mathbf{x})$ is approximated by Monte-Carlo. We optimize $h_{\tilde{f}}(\mathbf{x})$ with respect to $\mathbf{x}$ by using Bayesian optimization to the *stochastic* objective $h_{\tilde{f}}(\mathbf{x})$ (since $\tilde{f}$ is stochastic). We choose the duel $\mathbf{x}'_{next}$ as described in [5].

## References


[1] Mikkola, P., Todorović, M., Järvi, J., Rinke, P., and Kaski, S. (2020). Projective Preferential Bayesian Optimization. *In Proceedings of the* $37^{th}$ *International Conference on Machine Learning*, ICML'20.

[2] Ledoit, O., Wolf, M. (2004). Honey, I Shrunk the Sample Covariance Matrix. *The Journal of Portfolio Management* Jul 2004, 30 (4) p.110-119

[3] Arfaoui, M., Rezki, Z., Ghrayeb, A., Alouini, M. (2016). On the Secrecy Capacity of MISO Visible Light Communication Channels. *IEEE Global Communications Conference (GLOBECOM)* 2016, p.1-7

[4] The GPyOpt authors (2016). GPyOpt: A Bayesian Optimization framework in python. http://github.com/SheffieldML/GPyOpt.

[5] González, J., Dai, Z., Damianou, A., and Lawrence, N. D. (2017). Preferential Bayesian Optimization. *In Proceedings of the* $34^{th}$ *International Conference on Machine Learning*, ICML'17.

## PLOTS

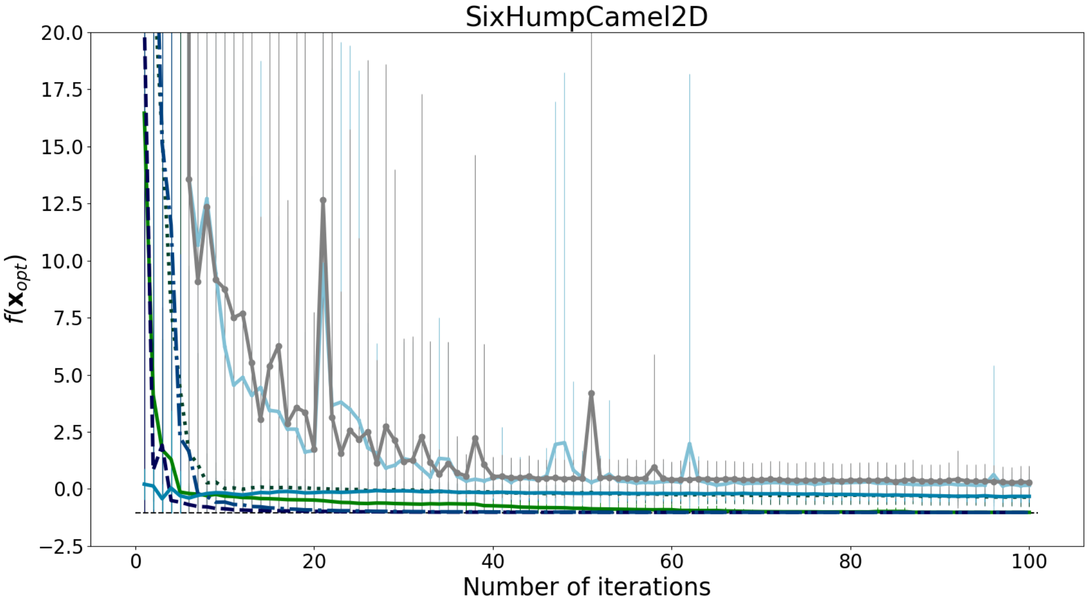

SixHumpCamel2D
$f(\mathbf{x}_{opt})$
20.0
17.5
15.0
12.5
10.0
7.5
5.0
2.5
0.0
−2.5
0
20
40
60
80
100
Number of iterations


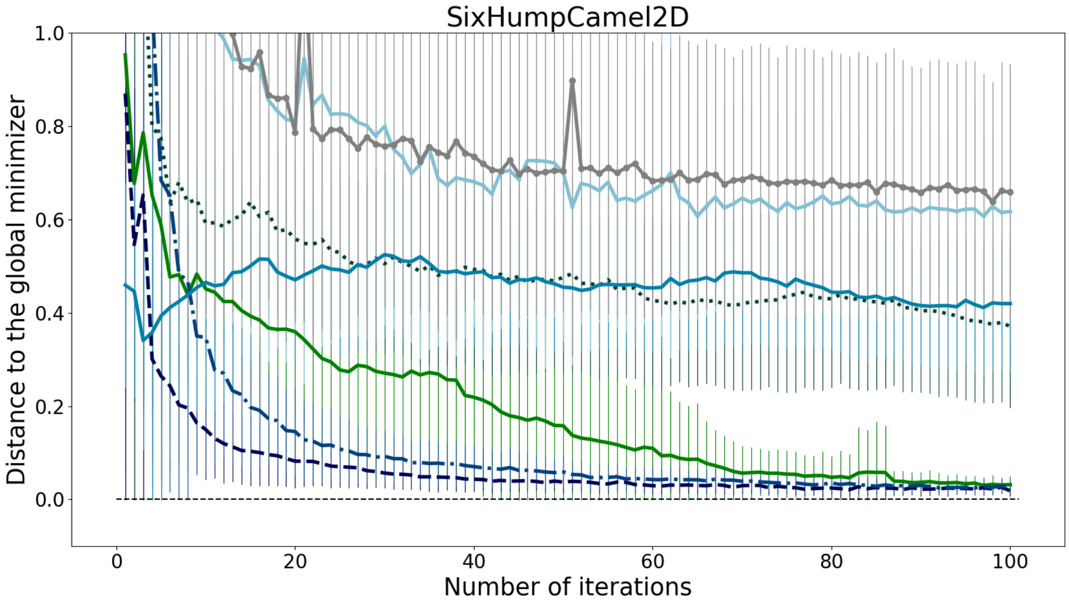

SixHumpCamel2D
Distance to the global minimizer
1.0
0.8
0.6
0.4
0.2
0.0
0
20
40
60
80
100
Number of iterations

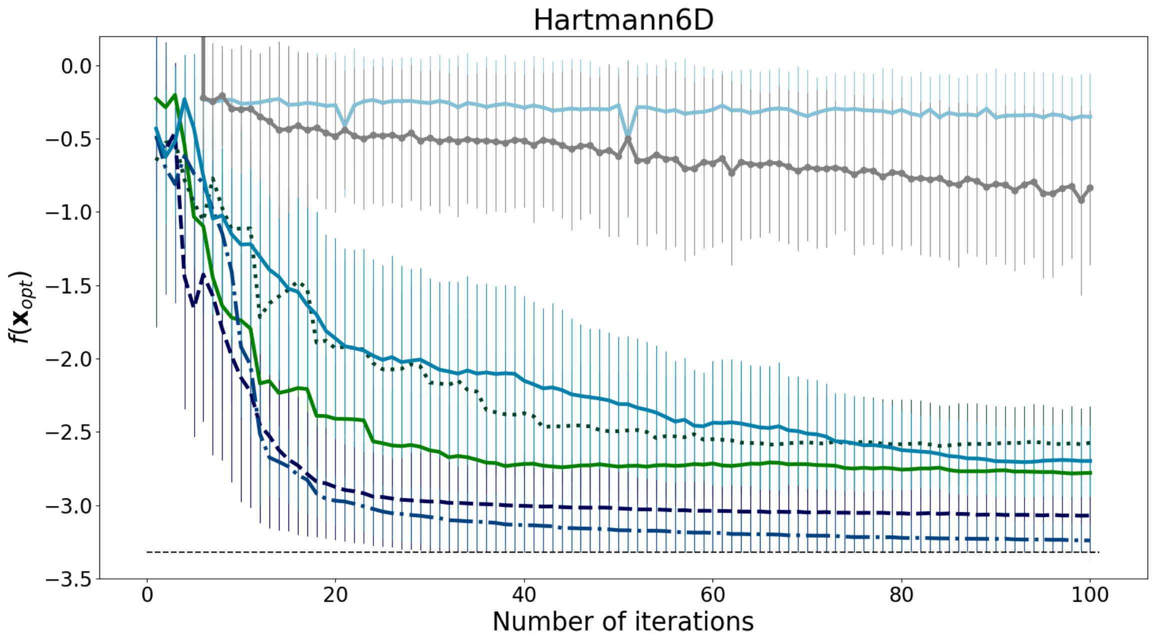
Hartmann6D
0.0
−0.5
−1.0
−1.5
−2.0
−2.5
−3.0
−3.5
$f(\mathbf{x}_{opt})$
0
20
40
60
80
100
Number of iterations

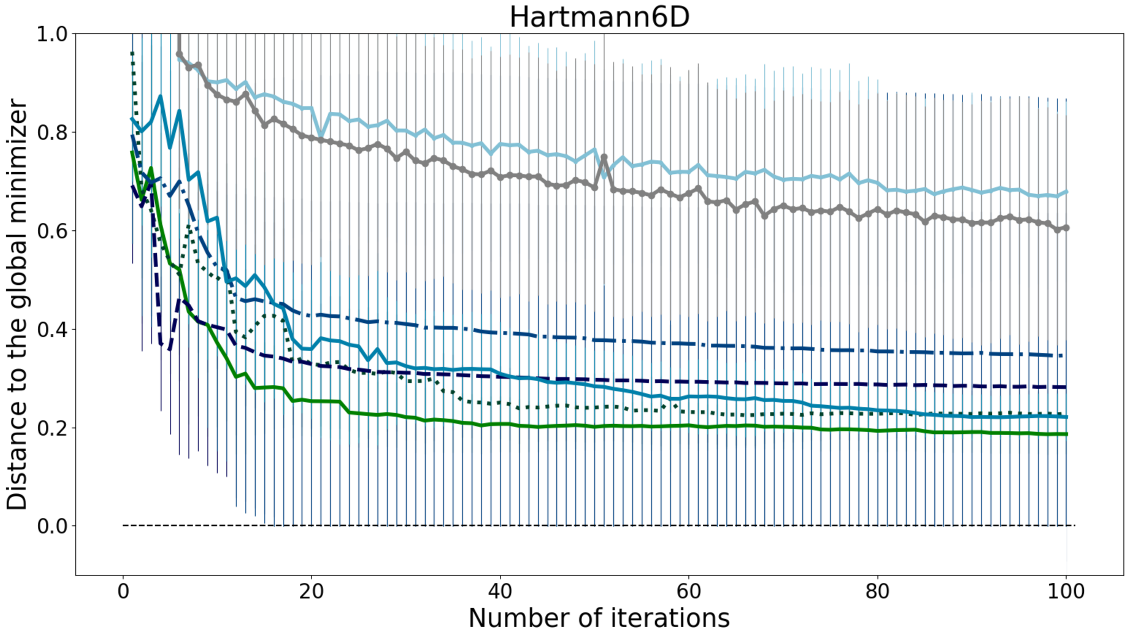
Hartmann6D
1.0
0.8
0.6
0.4
0.2
0.0
Distance to the global minimizer
0
20
40
60
80
100
Number of iterations

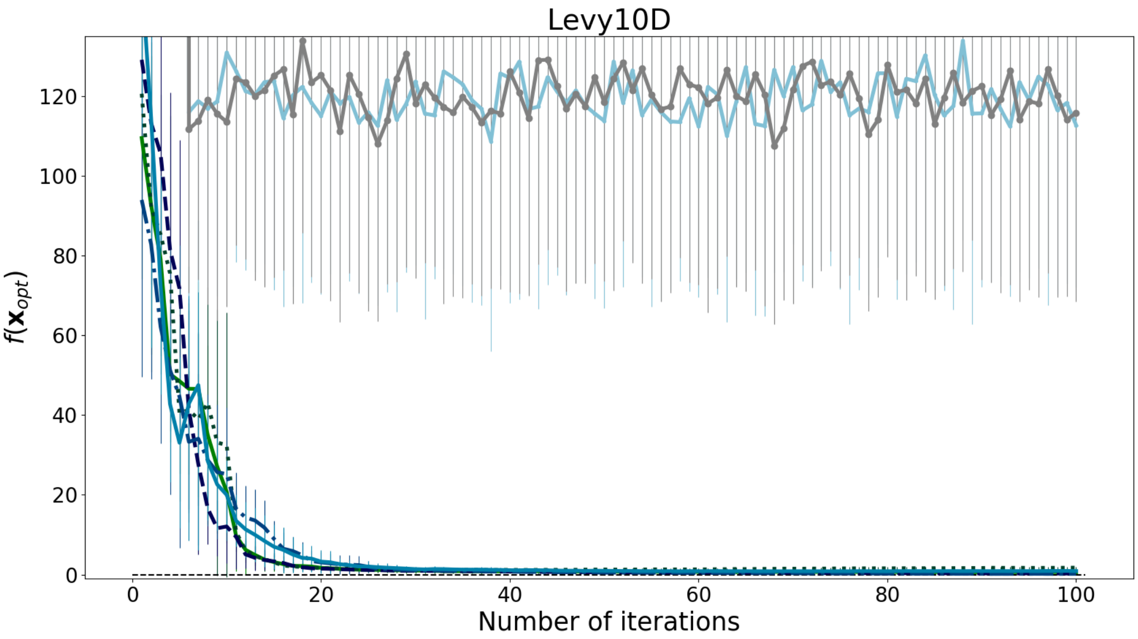
Levy10D
$f(\mathbf{x}_{opt})$
Number of iterations
0
20
40
60
80
100
120

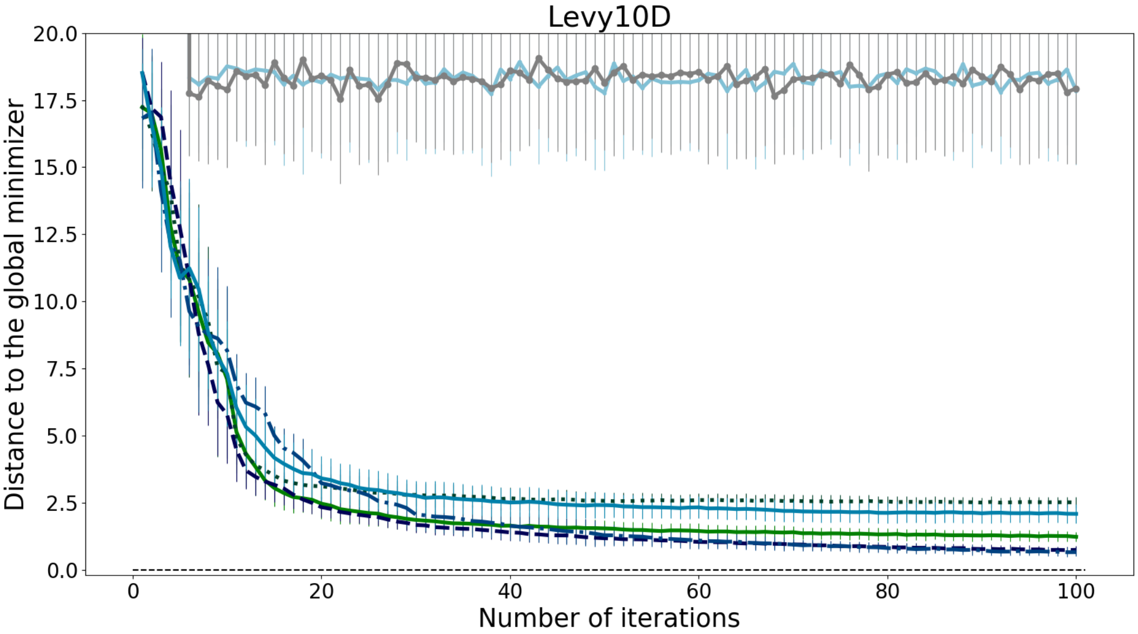
Levy10D
Distance to the global minimizer
Number of iterations
0.0
2.5
5.0
7.5
10.0
12.5
15.0
17.5
20.0
0
20
40
60
80
100

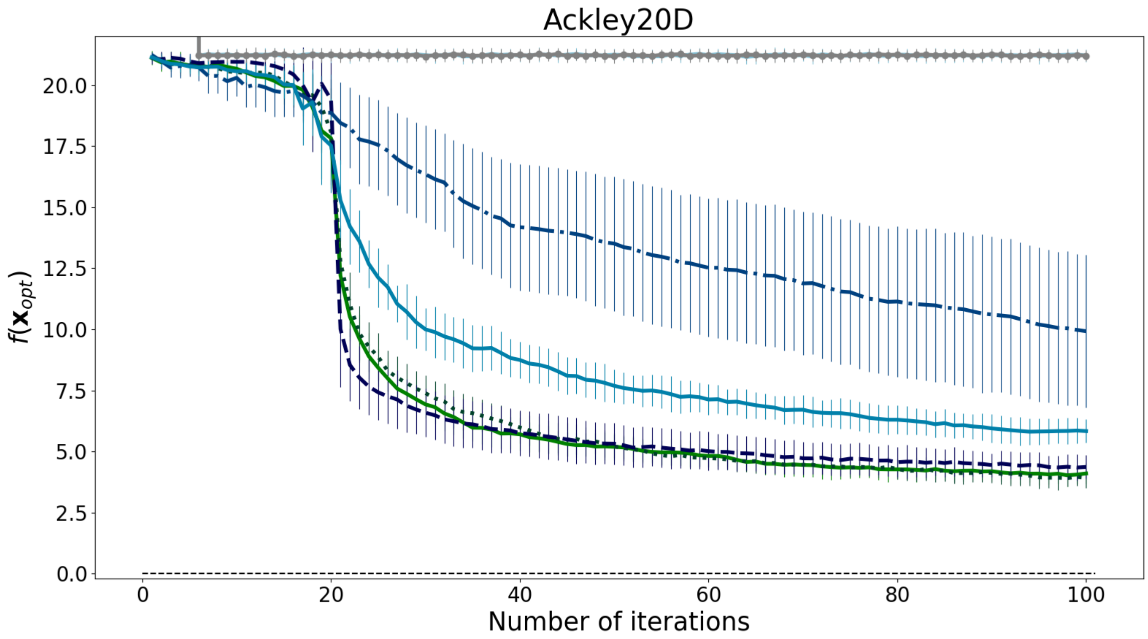
Ackley20D
f(x_opt)
20.0
17.5
15.0
12.5
10.0
7.5
5.0
2.5
0.0
0
20
40
60
80
100
Number of iterations

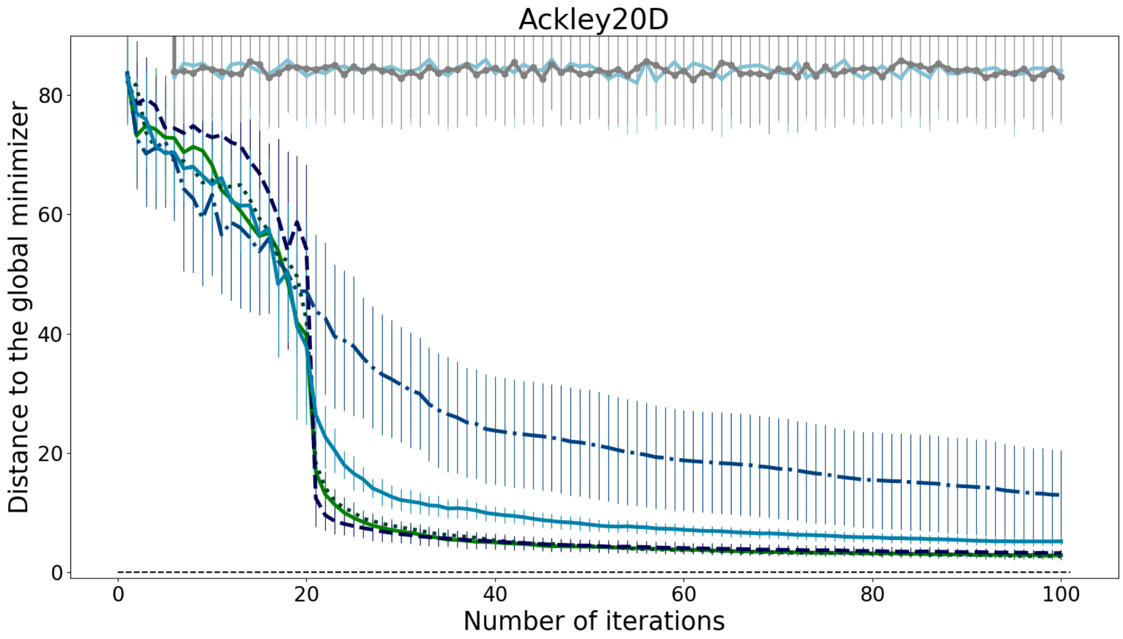
Ackley20D
Distance to the global minimizer
80
60
40
20
0
0
20
40
60
80
100
Number of iterations

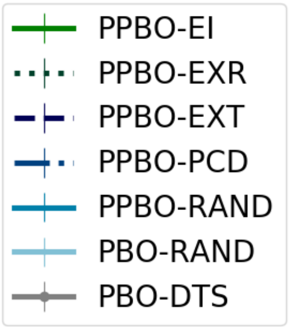


*Figure 1.* The meaning of the legends of the plots.
